# Supplementary material for: Semantic Consistency-Based Uncertainty Quantification for Factuality in Radiology Report Generation
Source: arXiv:2412.04606 source file (2025-03-16)
Supplement: Supplementary file 1 [file appendixa_v1.tex]

In this analysis, we grouped samples based on the presence of specific pathology findings to examine the correlation between UQ and GREEN for each subgroup. The overall correlation between UQ and GREEN is -0.52. However, for the Pneumothorax subgroup, the correlation is notably weaker at -0.08. This weak correlation is likely due to the underrepresentation of Pneumothorax in the dataset, comprising roughly 1\% of positive cases in the training set.
% \begin{table}[h!]
% \centering
% \small
% \begin{tabular}{l c}
% \hline
%     \textbf{Pathology Finding} & \textbf{Pearson Correlation (\%)} \\
%     \hline
%     No Finding & -68.44 \\
%     Enlarged Cardiomediastinum & -42.37 \\
%     Cardiomegaly & -35.07 \\
%     Lung Opacity & -38.84 \\
%     Lung Lesion & -41.47 \\
%     Edema & -34.01 \\
%     Consolidation & -43.60 \\
%     Pneumonia & -38.26 \\
%     Atelectasis & -42.91 \\
%     Pneumothorax & -8.09 \\
%     Pleural Effusion & -27.82 \\
%     Pleural Other & -40.04 \\
%     Fracture & -46.36 \\
%     Support Devices & -42.27 \\
%     \hline
% \end{tabular}
% \caption{Pearson correlation (as percentages) between UQ and GREEN across various subgroups of pathology findings.}
% \end{table}
